# Supplementary material for: DESI Strong Lens Foundry V: A Sample of HST-Observed Strong Lenses Modeled with GIGA-Lens
Source: arXiv:2512.07823 source file (2025-12-09)
Supplement: Supplementary file 1 [file appendix_magnif.tex]

% \subsection*{A. Magnification}\label{sec:magnif}

This section is an amplification of the appendix in \citep[][]{huang2025a} . We will explain in detail how magnification is calculated for the lensed arcs. We use three distinct methods, all consistent with each other. 

In the first method, we choose a luminosity threshold for the light. Such threshold is chosen so that each lensed arc or image is isolated from the other. The pixels in the source plane and the lens plane whose intensities exceed the threshold are selected, with both images being non-PSF convolved. The magnification for each arc is the ratio between the number of pixels of that arc and the number of pixels of the source, both above the chosen threshold.

\hspace{4mm}
However, this method requires an important adjustment. 
(\ed{MURT: this was in Saul/Nico's code but not explained in the Appendix of Paper I explicitly (DAG also feels this was not obvious, if not explained). XH will see if this extra explanation is necessary. })
If we had a continuous set of points in the lens and source planes, we would expect the brightest point in both planes to have the same value. Mathematically,
\begin{equation}
I(x_{b},y_{b})=I(\bar{x_{b}},\bar{y_{b}})
\label{eq:b_pixles}
\end{equation}
In equation \ref{eq:b_pixles}, b stands for brightest, $x,y$ are positions in the source plane, and $\bar{x}$, $\bar{y}$ are positions in the lens plane.

\hspace{4mm}
For a single point in the source plane with a specific intensity, the lens equation maps it to several points in the lens plane, keeping their intensity invariant. Then, it is clear that the increase in overall luminosity is due to the increase in area, not to the increase of the intensity of any point in the lens plane with respect to its equivalent in the source plane. %As a result, one should never expect to find a position in the lensed plane with intensity brighter than the brightest pixel in the source plane. 
\hspace{4mm}

In practice, we discretize the source and lens planes in a finite number of pixels with a particular size. In particular, we simulate the lens and source plane with pixels of the same size, $\delta_{I}$. Hence, the simulated images contain the counts in each pixel, not the value of $I(x,y)$ of each position $x,y$ inside the cutout. In this regard, we will denote a pixel by $\rho_{i}$ with $Light(\rho_{i})$ counts. As a consequence, the counts of the brightest pixel, $Light(\rho_{b})$, in the source and lens plane does not coincide by default, because our discretization is not accurate enough. This problem can be solved with the right corrections.

First, remember our objective is to achieve \ref{eq:b_pixles}. In our discretized planes, we can establish the following relation between the counts of each pixel and the intensity associated to each position: 

\begin{equation}
I(x,y)=Light(\rho_{i})/(\delta_{I})^{2}
\label{eq:light_position}
\end{equation}
\hspace{4mm}
The first correction is to make the grid in the source plane thinner by decreasing the size of the pixels, with side $\delta_{S}$. With this modification, from \ref{eq:light_position} we can obtain a new condition equivalent to \ref{eq:b_pixles}.

\begin{align}
 \frac{Light(\bar{\rho_{b}})}{(\delta_{S})^{2}}&=\frac{Light(\rho_{b})}{(\delta_{I})^{2}} \\
 Light(\bar{\rho_{b}})(\frac{\delta_{I}}{\delta_{S}})^{2}&=Light(\rho_{b})
\label{eq:brightest_pixel}
\end{align}

The previous expression leads to the second correction: after the source plane grid has been thinned, multiply the simulated image by $(\frac{\delta_{I}}{\delta_{S}})^{2}$.  With these two corrections, a suitable $\delta_{S}$ will satisfy \ref{eq:brightest_pixel}, or equivalently \ref{eq:b_pixles}. This can be checked by comparing the value of the brightest pixels in each plane. Once both values match, the magnification calculation methods can be applied. Figure \ref{fig:selected_pixels} shows the selected pixels in system \desionefivefour, with the two pertinent corrections in the source plane.

\begin{minipage}{\linewidth}
\begin{center}
    \includegraphics[keepaspectratio=true,scale=0.45]{figs/154figs/154_selected_pixels.png}
    \captionof{figure}{The selected pixels in the source plane and in each lensed image. The source plane has been plotted after undergoing the necessary corrections, which explains the difference in scale compared to the lens plane.}
    \label{fig:selected_pixels}
\end{center}
\end{minipage}

At last, one final correction is needed. Magnification is calculated as the ratio of areas in the source and lens plane. Counting pixels in each plane and dividing only works if the pixels in both planes have the same size. However, after the first correction, this isn't true anymore. Hence, the magnification is the ratio of pixels multiplied by the factor $(\frac{\delta_{I}}{\delta_{S}})^{2}$.

The second method does not require selecting an appropriate resolution in the source plane. In this case, we ray-trace to the source plane the central position (in arcseconds) of each pixel (within a non-PSF-convolved) that exceeds the same threshold than in the first method. Then, the area of the convex hull that encloses the delensed points is computed. The magnification for each lensed arc is the ratio between its area and the area of source area calculated this way. This method requires that the delensed positions in the source plane do not have concave features and the convex hull results in a reasonable enclosure. However, if the delensed source displays concavity but isn't too pronounced, computing the area using two convex hulls will give a reasonable enclosure. As an example, figures \ref{fig:convex_hull_B} and (\ref{fig:convex_hull_A}) are the convex hulls of system \desionefivefour.

\begin{minipage}{\linewidth}
\makebox[\linewidth]{
\includegraphics[keepaspectratio=true,scale=0.30]{figs/154figs/convex_hull_B.png}}
\captionof{figure}{This figure shows the convex hull that encloses the ray traced positions (in the source plane) of the pixels in the lensed image B in figure \ref{fig:scystem154}. Those pixels are displayed in the second plot of figure \ref{fig:selected_pixels}}
\label{fig:convex_hull_B}
\end{minipage}

\begin{minipage}{\linewidth}
\makebox[\linewidth]{
\includegraphics[keepaspectratio=true,scale=0.30]{figs/154figs/convex_hull_A.png}}
\captionof{figure}{This figure shows the two convex hulls which enclose the ray traced positions (in the source plane) of the pixels in the lensed image A in figure \ref{fig:scystem154}. Those pixels are displayed in the third plot of figure \ref{fig:selected_pixels}.In this case, estimating the area using two convex hulls was convenient, as the ray traced pixels create a concave shape.}
\label{fig:convex_hull_A}
\end{minipage}

\begin{figure}[H]
\centering
\begin{minipage}{0.48\linewidth}
    \includegraphics[width=\linewidth]{figs/154figs/convex_hull_B.png}
\end{minipage}
\hfill
\begin{minipage}{0.48\linewidth}
    \includegraphics[width=\linewidth]{figs/154figs/convex_hull_A.png}
\end{minipage}
\caption{Left: Convex hull enclosing the ray traced positions (in the source plane) of the pixels in lensed image B from Figure~\ref{fig:scystem154}, corresponding to the second plot in Figure~\ref{fig:selected_pixels}. \\
Right: Two convex hulls enclosing the ray traced positions of the pixels in lensed image A from Figure~\ref{fig:scystem154}, corresponding to the third plot in Figure~\ref{fig:selected_pixels}. Two hulls were used here due to the concave shape of the traced region.}
\label{fig:convex_hull_AB}
\end{figure}

Finally, the third method consists of applying the point-wise magnification function from Lenstronomy. The magnification for each arc is the median of the magnification of the pixels in the lensed arcs which exceed the chosen threshold. In our previous paper, we used the mean to estimate magnification. This is a reasonable choice if non of the lensed arcs sit over the critical curve where magnification is infinite. However, for systems where any lensed image sits on top of a critical curve, the median is a better metric.
